# Supplementary material for: SelEx: Self-Expertise in Fine-Grained Generalized Category Discovery
Source: arXiv:2408.14371 source file (2024-11-10)
Supplement: Supplementary file 5 [file Draft.tex]

\begin{equation}
\label{eq:eq8}
 \sum_{l\neq k}\frac{\hat{p}(z_j{=}l|\mathbf{c_i})}{\hat{p}(z_j{=}l)}{=}\sum_{l}\frac{\hat{p}(\mathbf{c_i}|z_j{=}l)}{\hat{p}(\mathbf{c_i})}{-}\frac{\hat{p}(z_j{=}k|\mathbf{c_i})}{\hat{p}(z_j{=}k)}\leq \frac{K}{\hat{p}(\mathbf{c_i})}{-}\frac{\hat{p}(z_j{=}k|\mathbf{c_i})}{\hat{p}(z_j{=}k)}
\end{equation}


Let's expand on $B$ using the inequality $ln(x+y)\leq ln(x)+\frac{y}{x},\text{ for }x,y>0$, we will have
Now assume a fraction of $\alpha$ samples of a category $\mathbf{c_i}$ are unlabelled. So we have: $\hat{p}(z_j{=}k|\mathbf{c_i}){\geq}\frac{1}{\alpha|\mathbf{c_i}|}$. If we use equation \cref{eq:eq7,eq:eq3,eq:eq8} we have:

Also we have $\hat{p}(z_j){=}{|z_j|\over N}$, 
Note that if our categories are balanced and we also ensure this balanced nature in training, we will have $\hat{p}(z_j)=\frac{1}{K}$ and $|\mathbf{c_i}|{=}\frac{N}{K}$, which converts the \cref{eq:eqA} to: 

\begin{equation}
\label{eq:eqAB}
\bar{\mathrm{A}}\leq-\ln\frac{K^2}{N\alpha}{=}-2\ln K+\ln\alpha+\ln N
\end{equation}
Now for the $\mathrm{B}$ part, since $\hat{p}(z_j{=}l|\mathbf{c_i})\leq\alpha$ and $\hat{p}(z_j{=}l){\geq}\frac{\underset{j}{\min}|z_j|}{N}$, we will have: 
\begin{equation}
\label{eq:eqB}
\mathrm{B}\leq\ln(\alpha NK)-\ln(\underset{j}{\min}|z_j|)
\end{equation}

Note that since we are considering the case where $\mathbf{c_i}{=}\mathbf{c_j}$ if $\mathbf{z_j}{\neq}\mathbf{c_i}$, the discrepancy between the model and true distribution in this scenario has been depicted in \cref{fig:sfig1}. As we can see from this figure $\frac{\hat{p}(z_j{=}k|\mathbf{c_i},Z)}{\hat{p}(z_j{=}k)}$ will be the intersection or purple area. 
While for unsupervised contrastive learning, we consider one positive sample and all other samples are negative, in supervised contrastive learning, there is a chance of more positive samples for each batch.
 
\begin{equation}
\label{eq:eqassingn}
\ln\hat{p}(y{=}1|\mathbf{c_i},z_j){=}{\hat{p}(y{=}1,\mathbf{c_i}, z_j)\over \hat{p}(\mathbf{c_i},z_j)}
\end{equation}
Since $\mathbf{c_i}$ is independent of $z_j$ we have $\hat{p}(\mathbf{c_i},z_j){=}\hat{p}(\mathbf{c_i})\hat{p}(z_j)$. Further we can consider that $\hat{p}(\mathbf{c_i}){=}{|\mathbf{c_i}|\over N}$ and $\hat{p}(z_j){=}{|z_j|\over N}$. Using \cref{fig:sfig1}, we can estimate $\hat{p}(y{=}1,\mathbf{c_i},z_j)$ as the ratio of the intersection between groundtruth label $\mathbf{c_i}$ and the assigned pseudolabel $z_j$. Let's show the number of samples in this section, which is the purple part in \cref{fig:sfig1} with $e_{kl}$ in which $k{=}\{\mathbf{c_i}\}_K$ and $l{=}\{z_j\}_K$. This is the number of samples with ground truth $k$, which the model classifies as $l$. 

%========================Start-Theorem==========================
\begin{theorem}
\label{theo:unsup}
 We will have the following upper bounds:
Both $i$ and ${j}$ are unlabelled
     \begin{align}  
\label{eq:upper}
    D_\mathrm{KL}[p(y|\mathbf{c_i},\mathbf{c_j})\parallel \hat{p}(y|\mathbf{x_i},\mathbf{x_j})]\leq 
    \ln K +\sum_{c_j}\mathcal{H}({|c_j|\over N}),
\end{align}
\end{theorem}
%========================End-Theorem==========================

Similarly, we can find that when $\mathbf{c_i}\neq\mathbf{c_j}$, we will have:
\begin{equation}
\label{eq:eq68}
 D_\mathrm{KL}[p(y|\mathbf{c_i},\mathbf{c_j}){\parallel} \hat{p}(y|\mathbf{c_i},z_j)]{=}-\ln \hat{p}(y{=}0|\mathbf{c_i},z_j),   
\end{equation}
This scenario has been depicted in \cref{fig:sfig2}. 

Since $\hat{p}(z_j{=}k|x_j){=}\frac{\hat{p}(z_j{=}k)\hat{p}(x_j|z_j=k)}{\hat{p}(x_j)}$ and $\hat{p}(x_j){=}\frac{1}{N}$, also if we consider the $\hat{p}(x_j|z_j=k)\sim \mathcal{N}(\mu_k,\sigma_k^2I)$ and since $\ln$ is concave, we will have: 
\begin{equation}
\label{eq:eq8}
 \sum_{k=1}^K\hat{p}(z_j{=}k|\mathbf{x_j})\ln\hat{p}(z_j{=}k){\leq}N\sum_{k=1}^K\hat{p}(z_j{=}k)e^{-\frac{||x_j-\mu_k||^2}{2\sigma_k^2}}\ln\hat{p}(z_j{=}k)
\end{equation}

\textbf{Intra-class Divergence:}\\
If $\mathbf{c_i}{=}\mathbf{c_j}$, we will have $p(y|\mathbf{c_i},\mathbf{c_j}){=}0$, according to \cref{eq:identy}. So we will have:
\begin{multline}
\label{eq:eq5}
 D_\mathrm{KL}[p(y|\mathbf{c_i},\mathbf{c_j}){\parallel} \hat{p}(y|\mathbf{c_i},\mathbf{c_j}, z_j{=}k)]{=}\\
 -\ln \hat{p}(y{=}1|\mathbf{c_i},\mathbf{c_j},z_j{=}k)\mathds{1}( \hat{p}(y{=}1|\mathbf{c_i},\mathbf{c_j},z_j{=}k){\neq}0)
\end{multline}
Note that here since we assume $\mathbf{c_j}{=}\mathbf{c_i}$, we can consider the value of the $\mathbf{c_j}$ as observed. 
In this equation $\mathds{1}( \hat{p}(y{=}1|\mathbf{c_i},z_j{=}k){\neq}0)$ ensures that only $k$s where $\hat{p}(y{=}1|\mathbf{c_i},z_j{=}k){\neq}0$ has been considered. We don't include this function in the next equations for simplicity but implicitly consider the condition it imposes on $k$.
Note that unlike \cite{oord2018representation}, we consider $\hat{p}(y)$ to be a Bernoulli distribution; this is because we only consider one sample at a time to see if this sample belongs to the same class or not. This is because, in their approach, categorical cross entropy forces the model to use one positive sample while considering all the remainder as negatives. But in the contrastive version, we can have multiple positives per each batch. Similar to \cite{oord2018representation}, we can write this probability as follows:
\begin{equation}
\label{eq:eqconp}
 \hat{p}(y=1|\mathbf{c_i}, \mathbf{c_j}, z_j{=}k){=}\frac{\frac{\hat{p}(z_j=k|\mathbf{c_i},\mathbf{c_j})}{\hat{p}(z_j=k)}}{\sum_{l=1}^K\frac{\hat{p}(z_j=l|\mathbf{c_i},\mathbf{c_j})}{\hat{p}(z_j=l)}}  
\end{equation}
Since when $y$ is unobserved, $z_j$ is independent of $\mathbf{c_i}$, Hence; we will have the following:
\begin{equation}
\label{eq:eq6}
 D_\mathrm{KL}[p(y|\mathbf{c_i},\mathbf{c_j}){\parallel} \hat{p}(y|\mathbf{c_i},\mathbf{c_j},z_j)]{=}\overbrace{-\ln\frac{\hat{p}(z_j{=}k|\mathbf{c_j})}{\hat{p}(z_j{=}k)}}^A+\underbrace{\ln\sum_{l=1}^K\frac{\hat{p}(z_j{=}l|\mathbf{c_j})}{\hat{p}(z_j{=}l)}}_B 
\end{equation}
To calculate $A$, since in \cref{eq:eq5}, the condition is that $\hat{p}(y{=}1|\mathbf{c_i},\mathbf{c_j},z_j{=}k){\neq}0$, we can conclude that $\hat{p}(z_j{=}k|\mathbf{c_j}){>}0$. At least one sample of $\mathbf{c_j}$ or $\mathbf{c_i}$ should have $z_j{=}k$, or else this probability will be zero. 
Assume a fraction of $\alpha_j$ samples of a category $\mathbf{c_j}$ are unlabelled. So we have: $\hat{p}(z_j{=}k|\mathbf{c_j}){\geq}\frac{1}{\alpha_j|\mathbf{c_j}|}$. Therefore, we can find an upper bound for $A$:
\begin{equation}
\label{eq:eqA1}
\mathrm{A}\leq \ln\alpha_j|\mathbf{c_j}|{+}\ln\hat{p}(z_j{=}k)
\end{equation}
To calculate $B$, since $\frac{\hat{p}(z_j{=}l|\mathbf{c_j})}{\hat{p}(z_j=l)}{=}\frac{\hat{p}(\mathbf{c_j}|z_j{=}l)}{\hat{p}(\mathbf{c_j})}$ and $\hat{p}(\mathbf{c_j}|z_j{=}l)\leq1$
\begin{equation}
\label{eq:eqB1}
\mathrm{B}\leq \ln\frac{K}{\hat{p}(\mathbf{c_j})}{=}\ln K-\ln\frac{|\mathbf{c_j}|}{N}
\end{equation}
If we use equation \cref{eq:eqB1,eq:eqA1} we have:
\begin{equation}
\label{eq:eq7}
 D_\mathrm{KL}[p(y|\mathbf{c_i},\mathbf{c_j}){\parallel} \hat{p}(y|\mathbf{c_i},\mathbf{c_j},z_j)]{\leq}\ln\hat{p}(z_j{=}k)+\ln\alpha_j NK
\end{equation}
Now if we replace this in \cref{eq:eq3}:
\begin{equation}
\label{eq:eqfinal}
D_\mathrm{KL}[p(y|\mathbf{c_i},\mathbf{c_j}){\parallel}\hat{p}(y|\mathbf{c_i},\mathbf{x_j})]{\leq}\ln\alpha_j NK+\sum_{k=1}^K\hat{p}(z_j{=}k|\mathbf{x_j})\ln\hat{p}(z_j{=}k)
\end{equation}
Note that since $\ln\hat{p}(z_j{=}k){\leq}0$, the second part is always negative. Hence, we will have:
\begin{equation}
\label{eq:eqcicj}
D_\mathrm{KL}[p(y|\mathbf{c_i},\mathbf{c_j}){\parallel}\hat{p}(y|\mathbf{c_i},\mathbf{x_j})]{\leq}\ln\alpha_j NK
\end{equation}
\textbf{Inter-class Divergence:}\\
Here we have $\mathbf{c_j}{\neq}\mathbf{c_i}$, we have a few changes from the previous part, particularly \cref{eq:eq5} will be as:
\begin{multline}
\label{eq:2eq5}
 D_\mathrm{KL}[p(y|\mathbf{c_i},\mathbf{c_j}){\parallel} \hat{p}(y|\mathbf{c_i},\mathbf{c_j}, z_j{=}k)]{=}\\
 -\ln \hat{p}(y{=}0|\mathbf{c_i},\mathbf{c_j},z_j{=}k)\mathds{1}( \hat{p}(y{=}0|\mathbf{c_i},\mathbf{c_j},z_j{=}k){\neq}0)
\end{multline}
Since we can consider $\hat{p}(y{=}0|\mathbf{c_i},\mathbf{c_j},z_j{=}k){=}1{-}\hat{p}(y{=}1|\mathbf{c_i},\mathbf{c_j},z_j{=}k)$, \cref{eq:eq6} becomes
\begin{equation}
\label{eq:2eq6}
 D_\mathrm{KL}[p(y|\mathbf{c_i},\mathbf{c_j}){\parallel} \hat{p}(y|\mathbf{c_i},\mathbf{c_j},z_j)]{=}\overbrace{-\ln\sum_{l\neq k}\frac{\hat{p}(z_j{=}l|\mathbf{c_j})}{\hat{p}(z_j{=}l)}}^A+\underbrace{\ln\sum_{l=1}^K\frac{\hat{p}(z_j{=}l|\mathbf{c_j})}{\hat{p}(z_j{=}l)}}_B 
\end{equation}
As in \cref{eq:2eqB1}
\begin{equation}
\label{eq:2eqB1}
\mathrm{B}\leq \ln\frac{K}{\hat{p}(\mathbf{c_j})}{=}\ln K-\ln\frac{|\mathbf{c_j}|}{N}
\end{equation}
We can also write $A$ as 
\begin{equation}
\label{eq:2eqA1}
\mathrm{A}\leq \ln\alpha_j|\mathbf{c_j}|{+}\ln\frac{1}{\sum_{l\neq k}\frac{1}{\hat{p}(z_j{=}l)}}
\end{equation}
From the harmonic and arithmetic mean inequality we know that $\frac{n}{\sum_{i=1}^nx_i^{-1}}{\leq}\frac{\sum_{i=1}^nx_i}{n}$
\begin{equation}
\label{eq:2eqA2}
\ln\frac{1}{\sum_{l\neq k}\frac{1}{\hat{p}(z_j{=}l)}}{\leq}\ln\frac{\sum_{l\neq k}\hat{p}(z_j{=}l)}{(K{-}1)^2}{=}\ln{(1{-}\hat{p}(z_j{=}k))}{-}2\ln{(K{-}1)}
\end{equation}
Considering the Maclaurin series for $\ln{(1{-}x)}$, we can write: 
\begin{equation}
\label{eq:2eqA3}
\mathrm{A}\leq \ln\alpha_j|\mathbf{c_j}|{-}\hat{p}(z_j{=}k){-}2\ln{(K{-}1)}
\end{equation}
Using \cref{eq:2eqB1,eq:2eqA3} we can rewrite \cref{eq:2eq6} as follows:
\begin{equation}
\label{eq:eq7}
 D_\mathrm{KL}[p(y|\mathbf{c_i},\mathbf{c_j}){\parallel} \hat{p}(y|\mathbf{c_i},\mathbf{c_j},z_j)]{\leq}\ln\hat{p}(z_j{=}k)+\ln\alpha_j NK
\end{equation}

\begin{equation}
\label{eq:2eqfinal}
D_\mathrm{KL}[p(y|\mathbf{c_i},\mathbf{c_j}){\parallel}\hat{p}(y|\mathbf{c_i},\mathbf{x_j})]{\leq}\ln\alpha_j NK+\sum_{k=1}^K\hat{p}(z_j{=}k|\mathbf{x_j})\ln\hat{p}(z_j{=}k)
\end{equation}

Let's name $\sum_{x_j{\in}\mathbf{c_j}}\hat{p}(x_j|z_j{=}k)$ as $V_{jk}$, which means the probability of samples which have a groundtruth $\{\mathbf{c_j}\}_K$ and are categorized $k$ by model. 

If we consider that $\hat{p}(x_j|z_j{=}k)\sim \mathcal{N}(\mu_k,\sum_k)$, the brace part is nonzero, hence, considering the Maclaurin series for $\ln{(1{+}x)}$, we can write: 
\begin{equation}
\label{eq:eqmac}
 D_\mathrm{KL}[p(y|\mathbf{c_i},\mathbf{c_j}){\parallel} \hat{p}(y|\mathbf{c_i},\mathbf{c_j},z_j)]{\leq}\frac{\sum_{l=1}^K\sum_{x_j{\in}\mathbf{c_j}}}
\end{equation}


\begin{multline}
\label{eq:eq6}
 D_\mathrm{KL}[p(y|\mathbf{c_i},\mathbf{c_j}){\parallel} \hat{p}(y|\mathbf{c_i},\mathbf{c_j},z_j)]{=}\overbrace{-\ln(\frac{N}{|c_j|}\sum_{x_j\in\mathbf{c_j}}\hat{p}(x_j|z_j{=}k))}^A+\\\underbrace{\ln(\frac{N}{|c_j|}\sum_{l=1}^K\sum_{x_j\in\mathbf{c_j}}\hat{p}(x_j|z_j{=}l)}_B 
\end{multline}


\begin{figure*}[t]
%\vspace{-2.5em}
%\begin{subfigure}
\begin{center}
\includegraphics[trim={0.2cm 8cm 9cm 0.2cm}, width=\linewidth]{Images/Main_fig_icml.pdf}
\end{center}
\vspace{-1.5em}
\caption{\textbf{Proposed framework for hierarchical contrastive learning.} Our method consists of three phases; in \textit{phase I}, our Hierarchical Semi-Supervised module extracts pseudo-labels for each hierarchy level. In \textit{phase II}, our hierarchical unsupervised contrastive module uses the negative samples from the same cluster as hard negatives for each hierarchy and distinguishes them from each other. Finally, in \textit{phase III}, our hierarchical supervised contrastive learning uses positives from the same cluster as weak positives for each hierarchy and aims to learn the higher-level similarities.}
\label{fig:modelframe}
\vspace{-0.3em}
\end{figure*}


Self-supervised learning has transformed the analysis of large-scale unlabeled data, but faces challenges in detailed data examination, often due to high false negative rates in contrastive learning-based methods. Our paper introduces 'Self-Expertise', a novel concept enhancing model complexity in recognizing distinctions, particularly in Generalized Category Discovery (GCD) – a task involving both identification of new categories and accurate classification of known ones. Initially, we use pseudo-labels to form basic clusters, offering 'soft supervision', which yields weaker, yet more frequent positive samples. This approach sets the foundation for the model to progressively address more intricate categorization tasks, enhancing adaptability to unfamiliar categories through shared abstractions. Simultaneously, a label smoothing parameter is implemented, pushing the model to refine intra-category differentiation at every abstraction level, ensuring distinct subcategory clustering within shared categories. This dual methodology incrementally augments the model's discrimination ability, in line with the Self-Expertise principle. Theoretical and empirical analyses confirm our method's superior performance over current leading techniques in GCD across diverse fine-grained datasets.





One reason for this might be that humans become experts in a way substantially different from machines. In contrast to machines, human expertise starts with overly general labels instead of overly specific ones. A human first learns what a 'bird is,' then what makes a bird a 'Grosbeak' and what makes a Grosbeak a 'Rose-breasted Grosbeak.' This approach to expertise has two advantages. First, there are more birds than grosbeaks, so there will be more positive samples for fast learning. Second, once we can distinguish a bird from a dog, for different bird species, it is more important to focus on distinguishing, for instance, a grosbeak from a finch rather than a dog. Distinguishing different bird species will be more challenging.
To learn from both data types simultaneously, separate classification heads~\cite{fini2021unified}, mixture model~\cite{zhong2021openmix}, and pseudo-labels~\cite{roy2022class} have been used.  The problem of encountering new classes at the test time has also been investigated in open-set recognition \cite{bendale2015towards, bendale2016towards,scheirer2012toward,vaze2021open}. In open-set recognition, the model aims to determine whether a sample is from a novel category or known category but not cluster instances into the correct novel categories.

The methodology proposed by \citet{vaze2022generalized} applies semi-supervised contrastive learning to generate a discriminative and informative embedding for both known and unknown categories. Initially, the method employs unsupervised contrastive learning to discern an image from a multitude of others. However, a noted limitation of unsupervised contrastive learning is its propensity to impose sometimes extreme augmentations as positive instances while treating visually similar samples as negatives, thereby driving the model to increase the distance between similar samples. To circumvent this issue, \citet{vaze2022generalized} integrate supervised contrastive learning into their approach, enabling the model to exploit the similarities among samples within the same class. This technique, however, is only applicable to known categories. Enhancing the model's reliance on supervised contrastive learning can improve the clustering quality for known categories at the expense of diminishing the performance of unknown category clusters and vice versa. Extreme reliance on either learning approach compromises the cluster purity for known and unknown categories.

There are several approaches to address the complex issue of unknown categories for machines, namely open-set recognition, novel class discovery, and generalized category discovery. 

\textbf{Open-Set Recognition}
 a primary strategy could involve discarding any novel category – in essence, dividing the data into known versus novel clusters while focusing on classifying known categories. This strategy is the well-studied problem of \textit{open set recognition} \cite{bendale2015towards, bendale2016towards,scheirer2012toward,vaze2021open}. 

How do humans become experts in a subject? When do we call a person an expert? "Expertise" is an abstract term that we use daily. Although there could be different approaches to defining this term, we can see expertise as the ability to discern minute differences in a topic of interest. For instance, a zoologist is more expert than a normal person in discerning birds because he can identify more finer details. It might be tempting to translate expertise to machines using supervised learning. While supervised learning outperforms humans in discerning finer details, for example, classifying images within many predefined categories \cite{he2016deep, krizhevsky2017imagenet, simonyan2014very, huang2017densely, szegedy2015going}, %. Despite their superior performance in familiar, well-defined settings, 
they fail when faced with the unknown, demonstrating a noticeable shortfall in generalization. However, an expert human can generalize unknown scenarios using knowledge from known ones. 

One reason for this might be that humans become experts in a way substantially different from machines. In contrast to machines, human expertise starts with overly general labels instead of overly specific ones. A human first learns what a 'bird is,' then what makes a bird a 'Grosbeak' and what makes a Grosbeak a 'Rose-breasted Grosbeak.' This approach to expertise has two advantages. First, there are more birds than grosbeaks, so there will be more positive samples for fast learning. Second, once we can distinguish a bird from a dog, for different bird species, it is more important to focus on distinguishing, for instance, a grosbeak from a finch rather than a dog. Distinguishing different bird species will be more challenging.

A widely accepted method to tackle unknown categories has been self-supervision. Interestingly, contrastive learning, a form of self-supervision, has demonstrated its potential in unearthing new semantics, suggesting an enticing path forward in the realm of discovering unknown categories. 
Despite recent advancements in adopting contrastive learning, a significant challenge persists due to the high occurrence of false negatives within the same category, which adversely impacts semantic clustering quality. The presence of a few false negatives from a category could result in the creation of a fragmented cluster for that category or, even more critically, the misassignment of samples to different clusters. 
For known category samples, supervised contrastive learning could potentially alleviate this issue for known categories with labeled data, thereby enhancing the discriminative capacity of the representation. Nonetheless, the challenge remains due to the absence of supervisory signals for novel categories. Due to these shortcomings, it has been shown recently that self-supervised learning is not suitable for fine-grained analysis. Recent studies, have attempted to address this issue through the utilization of intermediate concepts as a pseudo-supervisory mechanism. However, given their dependence on similarity graphs, these methods can be prone to sacrifice semantic similarity in favor of embedding similarity, thereby limiting their applicability for fine-grained categories where visually similar samples in the embedding can have different semantics.

\begin{table}[ht!]
%\vspace{-2em}
%\begin{table}
  \caption{\textbf{Effect of smoothing hyperparameter constant}. More smoothing means more reliance on the negative samples within the cluster which has a positive effect on novel categories.}
  \label{table:smoothing}
  \centering
  \resizebox{1\linewidth}{!}{
\begin{tabular}{l|ccc|ccc|ccc|ccc}
\toprule
&\multicolumn{3}{c}{\textbf{CUB-200}}  & \multicolumn{3}{c}{\textbf{FGVC-Aircraft}}&\multicolumn{3}{c}{\textbf{Stanford-Cars}}&\multicolumn{3}{c}{\textbf{Oxford-Pets}}\\ \cmidrule(lr){2-4} \cmidrule(lr){5-7} \cmidrule(lr){8-10} \cmidrule(lr){11-13}
 &All & Known  & Novel &  All & Known  & Novel&All & Known  & Novel&All & Known  & Novel\\
\midrule
%k-means \citep{arthur2007k}        & 52.0 & 52.2  & 50.8\\
$\alpha{=}0$  &62.6&71.9&58.2&&&&&& \\ % 51.3&	56.6&	48.7 \\
$\alpha{=}0.1$  & 72.4&\bf{76.2}&70.5&&&&&& \\
$\alpha{=}0.5$  &73.6 &75.3 &72.8&&&&&&\\
$\alpha{=}0.7$  &72.6&73.5 &72.2&&&&&&\\
$\alpha{=}1.0$ &\bf{74.9}&74.5&\bf{75.1}&&&&&&\\

\bottomrule
\end{tabular}}
%\end{table}
\end{table}



%Since the baseline already uses unsupervised and supervised contrastive learning, in Table \ref{tab:compseff}, for unsupervised contrastive learning, we consider its addition, which benefits from hierarchical label smoothing. 
%For supervised contrastive learning, we consider the version without any pseudo-labels as a baseline, while for our loss, we consider its hierarchical supervision using pseudo-labels.
%As we can see from this table, hierarchical semi-supervised k-means give the most improvement on both known and novel categories. Our unsupervised self-expertise $\mathcal{L}_{\text{HU}}$ benefits known categories. This aligns with our rationale for using this loss, given that known clusters have the supervision signals; they can attract semantically similar samples, which can be initially distant from each other in embedding space, and at the same time, our unsupervised self-expertise ignores the semantically similar negative samples that are distant from a particular sample, so overall these samples have no repel until they are in the same cluster. When we combine unsupervised self-expertise with the hierarchical semi-supervised k-means, these effects also translate to the novel categories because we have semantic labels. Meanwhile, our supervised self-expertise $\mathcal{L}_{\text{HS}}$ predictably has a strong positive effect on novel categories while also benefiting the known ones. This is because although hierarchies might benefit known categories, they already have reliable supervision in the form of labels. However, novel categories do not have ground-truth labels, and at finer granularities, pseudo-labels can be noisy. As we go up the hierarchy, the pseudo-labels for novel categories become more reliable and provide better supervision. Ultimately, the best result for both known and novel categories is obtained when all three components are combined.


\noindent\textbf{Generalization through Abstraction:}
One aspect of expertise is generalizing to unknown categories through shared abastractions. \textit{Novel class discovery} \cite{han2019learning, fini2021unified, xie2016unsupervised, han2020automatically, zhao2021novel, zhong2021openmix, joseph2022novel, roy2022class, rizve2022towards, zhao2021novel}, aims to categorize new categories, drawing on the understanding gained from known categories. However, it assumes mutual exclusivity between known and novel categories. A more pragmatic approach, and the focus of our work, involves uncovering novel categories concurrently with known ones. To address this concern, the concept of \textit{Generalized Category Discovery} \cite{pu2023dynamic, zhang2022promptcal, hao2023cipr, chiaroni2023parametric, wen2022simple, an2023generalized} has been introduced.
%\cs{What is the goal of this paragraph?}
The widely accepted method to tackle unknown categories has been self-supervision \cite{jaiswal2020survey,zhai2019s4l,liu2021self} through Contrastive learning \cite{chen2020simple, li2020prototypical, noroozi2016unsupervised,caron2018deep, cao2021open, han2020automatically}, which thrives on distinguishing between augmentation of a sample as positive vs all other samples as negatives. 
 However, the presence of a few false negatives from the same category could result in the creation of a fragmented cluster, which leads to the misassignment of samples to different categories \cite{caron2018deep, khorasgani2022slic, huynh2022boosting}. 
Supervised contrastive learning \cite{khosla2020supervised, vaze2022generalized} could potentially alleviate this issue for known categories with labeled data, thereby enhancing the discriminative capacity of the representation. Nonetheless, the challenge remains due to the absence of supervisory signals for unknown categories. 

\begin{wrapfigure}{r}{0.49\textwidth}
%{figure*}[ht]
\begin{subfigure}{.24\textwidth}
  \centering
  \resizebox{1\linewidth}{!}{
\begin{tikzpicture}
  % Overlapping blue cluster
  \draw[fill=red, opacity=0.2] (1.25,0) ellipse (1.25cm and 1cm);

  % First realistic cluster with smaller red circles around z_i
\draw[fill=blue, opacity=0.1] (0,0) circle (0.75cm);
  % Point z_i
  \filldraw [black] (0.5,0) circle (2pt) node[anchor=north] {$z_j$};

  % Second realistic cluster with smaller red circles around z_j
\draw[fill=blue, opacity=0.1] (2,0) circle (1cm);
  % Point z_j
  \filldraw [black] (2,0) circle (2pt) node[anchor=north] {$z_i$};
  \node at (0.9,0.5) {$k$};
\end{tikzpicture}}
  \caption{}
  \label{fig:sfig3}
\end{subfigure}
\begin{subfigure}{.24\textwidth}
  \centering
  \resizebox{1\linewidth}{!}{
\begin{tikzpicture}
  % Overlapping blue cluster
  \draw[fill=blue, opacity=0.1] (1.25,0) ellipse (1.25cm and 1cm);

  % First realistic cluster with smaller red circles around z_i
\draw[fill=red, opacity=0.2] (0,0) circle (0.75cm);
  % Point z_i
  \filldraw [black] (0.5,0) circle (2pt) node[anchor=north] {$z_j$};

  % Second realistic cluster with smaller red circles around z_j
\draw[fill=red, opacity=0.2] (2,0) circle (1cm);
  % Point z_j
  \filldraw [black] (2,0) circle (2pt) node[anchor=north] {${z_i}$};
  \node at (-0.25,0.5) {$k$};
  \node at (2.5,0.5) {$l$};

\end{tikzpicture}}
  \caption{}
  \label{fig:sfig4}
\end{subfigure}
\caption{\textbf{Different scenarios for two sample category variables.} The latent variables $z_i$ and $z_j$ are extracted from the model and corresponds to the images $i$ and $j$. In the figures, red assignments are done by model, while blue assignments are the ground truth category variable assignments. For unsupervised contrastive learning, neither of the labels is known, so the model makes a mistake if (a) $i$ and $j$ have different labels and are assigned to the same label $k$, (b) $i$ and $j$ have the same label, but model assign them to different labels $k$ and $l$.}
\label{fig:appclustersunsup}
%\label{fig:bays}
%\end{figure}
\end{wrapfigure}


\begin{figure*}[t!]
\vspace{1em}
\begin{subfigure}{.5\textwidth}
  \centering
  \resizebox{\textwidth}{!}{\begin{tikzpicture}
    \coordinate (origin) at (0, 0);

    \foreach[count=\i] \radius/\dim in {
                                        5.25/Aircraft,
                                        4.64/Standford-Cars,
                                        6.52/CUB,
                                        9.34/CIFAR10,
                                        7.05/CIFAR100,
                                        7.38/ImageNet}{
        \coordinate (\i) at (\i * 360 / 6: \radius);
        \node (title) at (\i * 360 / 6: 11) {\textbf{\Huge\dim}};
        \draw [line width=0.5mm](origin) -- (title);
    }
    \draw [line width=2mm,blue!80,opacity=.7] (1)
    \foreach \i in {2,...,6}{-- (\i)} --cycle;
     

        \foreach[count=\i] \radius/\dim in {
                                        5.23/Aircraft,
                                        4.06/Standford-Cars,
                                        6.21/CUB,
                                        9.85/CIFAR10,
                                        7.53/CIFAR100,
                                        7.83/ImageNet}{
        \coordinate (\i) at (\i * 360 / 6: \radius);
        %\node (title) at (\i * 360 / 6: 11) {\fontsize{50}{60}\dim};
        \draw [line width=0.5mm](origin) -- (title);
    }
        \draw [line width=2mm,green!80,opacity=.7] (1)
        \foreach \i in {2,...,6}{-- (\i)} --cycle;   

        %\foreach \i in {2,...,7}{-- (\i)} --cycle;  

        \foreach[count=\i] \radius/\dim in {
                                        5.33/Aircraft,
                                        5.14/Standford-Cars,
                                        7.28/CUB,
                                        9.48/CIFAR10,
                                        7.63/CIFAR100,
                                        7.78/ImageNet}{
        \coordinate (\i) at (\i * 360 / 6: \radius);
        %\node (title) at (\i * 360 / 6: 11) {\fontsize{50}{60}\dim};
        \draw [line width=0.5mm](origin) -- (title);
    }
        \draw [line width=2mm,red!80,opacity=.7] (1)
        \foreach \i in {2,...,6}{-- (\i)} --cycle;   

    %\draw [fill=blue, opacity=.7] (1)
    %                            \foreach \i in {2,...,7}{-- (\i)} --cycle;
                 
                                
\end{tikzpicture}}
  \caption{Novel}
  \label{fig:figr2}
\end{subfigure}
\begin{subfigure}{.5\textwidth}
  \centering
\resizebox{\textwidth}{!}{\begin{tikzpicture}
    \coordinate (origin) at (0, 0);

    \foreach[count=\i] \radius/\dim in {6.37/Aircraft,
                                        7.48/Standford-Cars,
                                        7.79/CUB,
                                        9.77/CIFAR10,
                                        8.22/CIFAR100,
                                        9.38/ImageNet}{
        \coordinate (\i) at (\i * 360 / 6: \radius);
        \node (title) at (\i * 360 / 6: 12) {\textbf{\Huge\dim}};
        \draw [line width=0.5mm](origin) -- (title);
    }
    \draw [line width=2mm,blue!80,opacity=.7] (1)
    \foreach \i in {2,...,6}{-- (\i)} --cycle;

        \foreach[count=\i] \radius/\dim in {5.22/Aircraft,
                                        7.01/Standford-Cars,
                                        6.44/CUB,
                                        9.66/CIFAR10,
                                        8.42/CIFAR100,
                                        9.27/ImageNet}{
        \coordinate (\i) at (\i * 360 / 6: \radius);
        %\node (title) at (\i * 360 / 6: 11) {\Huge\dim};
        \draw [line width=0.5mm](origin) -- (title);
    }
        \draw [line width=2mm,green!80,opacity=.7] (1)
        \foreach \i in {2,...,6}{-- (\i)} --cycle;   

        %\foreach \i in {2,...,7}{-- (\i)} --cycle;  

        \foreach[count=\i] \radius/\dim in {
                                        6.47/Aircraft,
                                        7.54/Standford-Cars,
                                        7.53/CUB,
                                        9.81/CIFAR10,
                                        8.53/CIFAR100,
                                        9.36/ImageNet}{
        \coordinate (\i) at (\i * 360 / 6: \radius);
        %\node (title) at (\i * 360 / 6: 11) {\fontsize{50}{60}\dim};
        \draw [line width=0.5mm](origin) -- (title);
    }
        \draw [line width=2mm,red!80,opacity=.7] (1)
        \foreach \i in {2,...,6}{-- (\i)} --cycle;   

    %\draw [fill=blue, opacity=.7] (1)
    %                            \foreach \i in {2,...,7}{-- (\i)} --cycle;
                       
\end{tikzpicture}}
  \caption{Known}
  \label{fig:figr3}
\end{subfigure}
\vspace{-2em}
\caption{\textbf{Comparative Radar Chart of Model Performances Across Diverse Datasets:} This visualization showcases the benchmarking of various models on different types of datasets. The green graph represents PromptCAL \cite{zhang2022promptcal}, the current state-of-the-art (SOTA) model for coarse-grained datasets. The blue graph indicates the performance of Infosieve \cite{rastegar2023learn}, which achieves SOTA results on fine-grained datasets. The red line highlights our proposed model's performance. The chart is segmented into two main categories for analysis: \textit{(a) Novel categories}, \textit{(b) Known categories} \ya{add intermediate ticks, such that it's a nicer spider plot. you can also choose the axis-offset, such that the differences become bigger.}}
\vspace{-2em}
\label{fig:radar}
\end{figure*}

%========================Start-Figure==========================

\begin{wrapfigure}{r}{0.45\textwidth}
\vspace{-3.5em}
\includegraphics[width=\linewidth]{Images/clusters.png}

\caption{\small{\textbf{Unsupervised Self-Expertise.} Our method maximizes repulsive forces between samples of the same category, such as cats, at lower levels of pseudo-label hierarchy. This design ensures that a misclassified sample, such as a lion, is effectively expelled from the incorrect cluster. Conversely, suppose a correct cat sample is erroneously expelled. In that case, it will likely be re-attracted to the appropriate cluster due to stronger repulsive forces from clusters of semantically dissimilar categories. \ya{figure is similar to fig1 and also does not really tell the reader anything new. what would be convincing is actually showing the story that you tell here in an actual experiment.}} %\cs{This figure resembles Figure 1 too much, why needed to repeat?} }
}\label{fig:clusters}
\vspace{-2em}
\end{wrapfigure}
%========================End-Figure=========================='


\begin{figure*}[t!]
\vspace{1em}
\begin{subfigure}{.5\textwidth}
  \centering
  \resizebox{\textwidth}{!}{\begin{tikzpicture}
    \coordinate (origin) at (0, 0);

    \foreach[count=\i] \radius/\dim in {
                                        5.25/Aircraft,
                                        4.64/Standford-Cars,
                                        6.52/CUB,
                                        9.34/CIFAR10,
                                        7.05/CIFAR100,
                                        7.38/ImageNet}{
        \coordinate (\i) at (\i * 360 / 6: \radius);
        \node (title) at (\i * 360 / 6: 11) {\textbf{\Huge\dim}};
        \draw [line width=0.5mm](origin) -- (title);
    }
    \draw [line width=2mm,blue!80,opacity=.7] (1)
    \foreach \i in {2,...,6}{-- (\i)} --cycle;
     

        \foreach[count=\i] \radius/\dim in {
                                        5.23/Aircraft,
                                        4.06/Standford-Cars,
                                        6.21/CUB,
                                        9.85/CIFAR10,
                                        7.53/CIFAR100,
                                        7.83/ImageNet}{
        \coordinate (\i) at (\i * 360 / 6: \radius);
        %\node (title) at (\i * 360 / 6: 11) {\fontsize{50}{60}\dim};
        \draw [line width=0.5mm](origin) -- (title);
    }
        \draw [line width=2mm,green!80,opacity=.7] (1)
        \foreach \i in {2,...,6}{-- (\i)} --cycle;   

        %\foreach \i in {2,...,7}{-- (\i)} --cycle;  

        \foreach[count=\i] \radius/\dim in {
                                        5.33/Aircraft,
                                        5.14/Standford-Cars,
                                        7.28/CUB,
                                        9.48/CIFAR10,
                                        7.63/CIFAR100,
                                        7.78/ImageNet}{
        \coordinate (\i) at (\i * 360 / 6: \radius);
        %\node (title) at (\i * 360 / 6: 11) {\fontsize{50}{60}\dim};
        \draw [line width=0.5mm](origin) -- (title);
    }
        \draw [line width=2mm,red!80,opacity=.7] (1)
        \foreach \i in {2,...,6}{-- (\i)} --cycle;   

    %\draw [fill=blue, opacity=.7] (1)
    %                            \foreach \i in {2,...,7}{-- (\i)} --cycle;
                 
                                
\end{tikzpicture}}
  \caption{Novel}
  \label{fig:figr2}
\end{subfigure}
\begin{subfigure}{.5\textwidth}
  \centering
\resizebox{\textwidth}{!}{\begin{tikzpicture}
    \coordinate (origin) at (0, 0);

    \foreach[count=\i] \radius/\dim in {6.37/Aircraft,
                                        7.48/Standford-Cars,
                                        7.79/CUB,
                                        9.77/CIFAR10,
                                        8.22/CIFAR100,
                                        9.38/ImageNet}{
        \coordinate (\i) at (\i * 360 / 6: \radius);
        \node (title) at (\i * 360 / 6: 12) {\textbf{\Huge\dim}};
        \draw [line width=0.5mm](origin) -- (title);
    }
    \draw [line width=2mm,blue!80,opacity=.7] (1)
    \foreach \i in {2,...,6}{-- (\i)} --cycle;

        \foreach[count=\i] \radius/\dim in {5.22/Aircraft,
                                        7.01/Standford-Cars,
                                        6.44/CUB,
                                        9.66/CIFAR10,
                                        8.42/CIFAR100,
                                        9.27/ImageNet}{
        \coordinate (\i) at (\i * 360 / 6: \radius);
        %\node (title) at (\i * 360 / 6: 11) {\Huge\dim};
        \draw [line width=0.5mm](origin) -- (title);
    }
        \draw [line width=2mm,green!80,opacity=.7] (1)
        \foreach \i in {2,...,6}{-- (\i)} --cycle;   

        %\foreach \i in {2,...,7}{-- (\i)} --cycle;  

        \foreach[count=\i] \radius/\dim in {
                                        6.47/Aircraft,
                                        7.54/Standford-Cars,
                                        7.53/CUB,
                                        9.81/CIFAR10,
                                        8.53/CIFAR100,
                                        9.36/ImageNet}{
        \coordinate (\i) at (\i * 360 / 6: \radius);
        %\node (title) at (\i * 360 / 6: 11) {\fontsize{50}{60}\dim};
        \draw [line width=0.5mm](origin) -- (title);
    }
        \draw [line width=2mm,red!80,opacity=.7] (1)
        \foreach \i in {2,...,6}{-- (\i)} --cycle;   

    %\draw [fill=blue, opacity=.7] (1)
    %                            \foreach \i in {2,...,7}{-- (\i)} --cycle;
                       
\end{tikzpicture}}
  \caption{Known}
  \label{fig:figr3}
\end{subfigure}
\vspace{-2em}
\caption{\textbf{Comparative Radar Chart of Model Performances Across Diverse Datasets:} This visualization showcases the benchmarking of various models on different types of datasets. The green graph represents PromptCAL \cite{zhang2022promptcal}, the current state-of-the-art (SOTA) model for coarse-grained datasets. The blue graph indicates the performance of Infosieve \cite{rastegar2023learn}, which achieves SOTA results on fine-grained datasets. The red line highlights our proposed model's performance. The chart is segmented into two main categories for analysis: \textit{(a) Novel categories}, \textit{(b) Known categories} \ya{add intermediate ticks, such that it's a nicer spider plot. you can also choose the axis-offset, such that the differences become bigger.}}
\vspace{-2em}
\label{fig:radar}
\end{figure*}


\begin{wraptable}{r}{0.4\textwidth}
\vspace{-2em}
%\begin{table}
  \caption{\textbf{Effect of smoothing hyperparameter constant}. More smoothing means more reliance on the negative samples within the cluster which has a positive effect on novel categories.}
  \label{table:smoothingconst}
    \centering
\resizebox{0.87\linewidth}{!}{

\begin{tabular}{lccc}
\toprule
% \multicolumn{4}{c}{\textbf{Smoothing Hyperparameter Constant}}\\ \cmidrule(lr){1-4}%{2-4}
\textbf{Method}  &  All & Known  & Novel\\
\midrule
%k-means \citep{arthur2007k}        & 52.0 & 52.2  & 50.8\\
Baseline   &62.6&71.9&58.2 \\ % 51.3&	56.6&	48.7 \\
$\alpha{=}0.1$  & 72.4&\bf{76.2}&70.5 \\
$\alpha{=}0.2$  &70.9 &73.1 &69.8\\
$\alpha{=}0.3$  &70.1 &72.1 &69.1\\
$\alpha{=}0.4$ &71.6 &73.7 &70.5\\
$\alpha{=}0.5$  &73.6 &75.3 &72.8\\
$\alpha{=}0.6$ &71.0&74.3&69.3\\
$\alpha{=}0.7$  &72.6&73.5 &72.2\\
$\alpha{=}0.8$  &74.3&73.9 &74.5\\
$\alpha{=}0.9$  &73.7 &74.3 &73.4\\
$\alpha{=}1.0$ &\bf{74.9}&74.5&\bf{75.1}\\

\bottomrule
\end{tabular}}
\vspace{-2em}
%\end{table}
\end{wraptable}


\begin{tikzpicture}
    \coordinate (origin) at (0, 0);

    \foreach[count=\i] \radius/\dim in {6.37/Aircraft,
                                        7.48/Standford-Cars,
                                        7.79/CUB,
                                        9.77/CIFAR10,
                                        8.22/CIFAR100,
                                        9.38/ImageNet}{
        \coordinate (\i) at (\i * 360 / 6: \radius);
        \node (title) at (\i * 360 / 6: 12) {\textbf{\Huge\dim}};
        \draw [line width=0.5mm](origin) -- (title);
    }
    \draw [line width=2mm,blue!80,opacity=.7] (1)
    \foreach \i in {2,...,6}{-- (\i)} --cycle;

        \foreach[count=\i] \radius/\dim in {5.22/Aircraft,
                                        7.01/Standford-Cars,
                                        6.44/CUB,
                                        9.66/CIFAR10,
                                        8.42/CIFAR100,
                                        9.27/ImageNet}{
        \coordinate (\i) at (\i * 360 / 6: \radius);
        %\node (title) at (\i * 360 / 6: 11) {\Huge\dim};
        \draw [line width=0.5mm](origin) -- (title);
    }
        \draw [line width=2mm,green!80,opacity=.7] (1)
        \foreach \i in {2,...,6}{-- (\i)} --cycle;   

        %\foreach \i in {2,...,7}{-- (\i)} --cycle;  

        \foreach[count=\i] \radius/\dim in {
                                        6.47/Aircraft,
                                        7.54/Standford-Cars,
                                        7.53/CUB,
                                        9.81/CIFAR10,
                                        8.53/CIFAR100,
                                        9.36/ImageNet}{
        \coordinate (\i) at (\i * 360 / 6: \radius);
        %\node (title) at (\i * 360 / 6: 11) {\fontsize{50}{60}\dim};
        \draw [line width=0.5mm](origin) -- (title);
    }
        \draw [line width=2mm,red!80,opacity=.7] (1)
        \foreach \i in {2,...,6}{-- (\i)} --cycle;   

    %\draw [fill=blue, opacity=.7] (1)
    %                            \foreach \i in {2,...,7}{-- (\i)} --cycle;
                       
\end{tikzpicture}

Nonetheless, a lower $K$ may lead to an increase in $\mathcal{H}(x|z)$. Considering a scenario where the distribution of $x$ for each $z$ adheres to a spherical Gaussian with a standard deviation denoted by $\sigma_K$ (here, $K$ represents the total number of categories in the dataset), we observe the following relationship,
%%========================Start-Equation==========================
%\begin{align}  
%\label{eq:uppergaussmain}
%    \mathcal{H}(x|z){=}\mathcal{C}{+}\ln \sigma_K,
%\end{align}
%========================End-Equation==========================
where $\mathcal{C}$ is a constant independent of $K$. In the Appendix, we demonstrate that $\sigma_{\frac{K}{2}} {<}2\sigma_K$, implying that a reduction in $K$ within \cref{eq:uppermain} results in a lower overall upper bound



Let's show this upper bound by $\mathcal{U}_K$. For $\frac{K}{2}$ categories we will have:
%========================Start-Equation==========================
\begin{equation}
\label{eq:Uk2}
    \mathcal{U}_\frac{K}{2}{=}\frac{K^2}{4}\ln\frac{N}{K}{+}\frac{K^2}{4}\ln 2{=}\frac{\mathcal{U}_{K}}{4}{+}\frac{K^2}{4}\ln 2
\end{equation}
%========================End-Equation==========================
we consider the hierarchical categories and show the upper bound with $\hat{\mathcal{U}}_K$ we will have $\hat{\mathcal{U}}_K=\frac{K^2}{2}\ln{N}{K}$ which is not useful.


In this work, we address Generalized Category Discovery, focusing on the simultaneous identification of novel categories and accurate classification of known ones. Traditional approaches, primarily reliant on self-supervision and contrastive learning, often struggle with fine-grained distinctions. To overcome this, we introduce `self-expertise,' which enhances the model's capability to make increasingly finer distinctions while being able to identify unknown categories. To this end, we adopt unsupervised self-expertise to refine the distinctions and supervised self-expertise to enhance generalization. Our approach begins with hierarchical pseudo-labeling, providing initial `soft supervision' for the model's supervised and unsupervised self-expertise components. In comparison to traditional supervised contrastive learning, these pseudo-labels yield more abstract and weak yet frequent, positive samples and more abstract yet stronger negative samples to form initial clusters that are generalizable to unknown categories through shared abstractions. In addition, contrary to traditional unsupervised contrastive learning, we propose unsupervised self-expertise, which guides the model to refine its within-category distinctions at each level of abstraction by focusing on within-category samples as hard negatives instead of all samples.
Motivated by our theoretical analyses, our empirical evidence demonstrates that our approach outperforms state-of-the-art methods in Generalized Category Discovery across multiple fine-grained datasets.


rewrite \cref{eq:dlmain} as:
%========================Start-Equation==========================
\begin{align}
\label{eq:expandmain}
    D_\mathrm{KL}[p(y|\mathbf{c_i},\mathbf{c_j}){\parallel}\hat{p}(y|\mathbf{c_i},\mathbf{x_j})]=&D_\mathrm{KL}[p(y|\mathbf{c_i},\mathbf{c_j})
    {\parallel}\sum_{z_j=1}^K\hat{p}(z_j|\mathbf{x_j})\hat{p}(y|\mathbf{c_i},z_j)]\\ 
    \leq&\sum_{z_j=1}^K\hat{p}(z_j|\mathbf{x_j})D_\mathrm{KL}[p(y|\mathbf{c_i},\mathbf{c_j}){\parallel} \hat{p}(y|\mathbf{c_i},z_j)],
\end{align}
%========================End-Equation========================== 
Which 

In this paper, we address Generalized Category Discovery, aiming to simultaneously uncover novel categories and accurately classify known ones. Traditional methods, which lean heavily on self-supervision and contrastive learning, often fall short when distinguishing between fine-grained categories. Our novel solution introduces the concept of `self-expertise', a mechanism designed to improve the model's ability to discern increasingly subtle differences and identify previously unknown categories. Our method employs both unsupervised and supervised self-expertise techniques: the former refines subtle distinctions within categories, and the latter bolsters the model's generalization capabilities. This process initiates with hierarchical pseudo-labeling to provide `soft supervision', enhancing both the supervised and unsupervised aspects of self-expertise. Our supervised self-expertise contrasts with traditional supervised contrastive learning by adopting more abstract yet frequent positive samples as `weak' positives while more abstract negative samples as `strong' negatives, establishing initial clusters that can generalize to novel categories through shared abstractions. Furthermore, our unsupervised self-expertise diverges from conventional unsupervised contrastive learning,  by compeling the model to refine its internal category distinctions at each abstraction level by treating within-category examples as `hard' negatives. 

Supported by theoretical insights, our empirical results showcase that our method outperforms existing state-of-the-art techniques in Generalized Category Discovery across several fine-grained datasets


In this paper, we introduce a novel Generalized Category Discovery methodology that leverages the strengths of contrastive learning and pseudo-labeling to effectively identify unknown categories by progressively developing self-expertise. In general, `expertise' can be defined as the ability to generalize across varying levels of abstraction, ranging from coarse to fine. This concept mirrors, for example, the proficiency of an ornithologist, who not only identifies novel species across different abstraction levels but also distinguishes between species within each level, a skill beyond the capability of an average person. In essence, expertise can be defined by two core components: discerning fine details and abstract generalization. This idea, illustrated in \cref{fig:fig}, showcases how unsupervised self-expertise enhances our ability to perceive subtle nuances while supervised self-expertise facilitates our capacity for generalization. In this paper, we make four contributions:


%========================Start-Figure==========================

\begin{wrapfigure}{r}{0.45\textwidth}
\vspace{-3.5em}
\includegraphics[width=\linewidth]{Images/clusters.png}

\caption{\small{\textbf{Unsupervised Self-Expertise.} Our method maximizes repulsive forces between samples of the same category, such as cats, at lower levels of pseudo-label hierarchy. This design ensures that a misclassified sample, such as a lion, is effectively expelled from the incorrect cluster. Conversely, suppose a correct cat sample is erroneously expelled. In that case, it will likely be re-attracted to the appropriate cluster due to stronger repulsive forces from clusters of semantically dissimilar categories. \ya{figure is similar to fig1 and also does not really tell the reader anything new. what would be convincing is actually showing the story that you tell here in an actual experiment.}} %\cs{This figure resembles Figure 1 too much, why needed to repeat?} }
}\label{fig:clusters}
\vspace{-2em}
\end{wrapfigure}
%========================End-Figure==========================

proposed by Han \etal~\cite{han2019learning} focuses on the transfer of classification knowledge from known to novel categories. Initial approaches \cite{han2019deep, hsu2017learning, hsu2019multi} adopted a two-stage methodology, where representation learning was confined to labeled data in the first stage, followed by the transfer of learned category structures to unknown categories in the subsequent stage. Recent advancements, have shifted towards a more integrated, single-stage approach, \eg,~\cite{fini2021unified, han2020automatically, zhao2021novel, zhong2021openmix, roy2022class, rizve2022towards}, where both labeled and unlabeled data are utilized concurrently for representation learning. Despite these developments, a fundamental challenge persists in the novel category discovery: the assumption of mutual exclusivity between known and novel categories.  In our work, we focus on the pragmatic approach of uncovering both novel and known categories concurrently. 


\begin{algorithm}[ht]
%\cs{Move to supplemental?}
   \caption{Balanced Semi-Supervised Kmeans (BSSK)}
   \label{alg:BSSK}
   \begin{algorithmic}[1]
       \REQUIRE Cluster size $C$, Initial centers $\mu^1, \ldots, \mu^K$
       \ENSURE Pseudo-labels for unlabeled data
       \FOR{$iter = 1$ \TO $n_{iter}$}
           \STATE Assign each data point $x_j$ to the closest cluster center.
           \FOR{$k = 1$ \TO $K$}
               \STATE Sort samples in cluster $c^k$ by their distance to center $\mu^k$.
               \STATE Compute the number of samples in cluster $|c^k|$.
               \IF{$|c^k| > C$}
                   \STATE Keep the $C$ closest samples in $c^k$, mark the rest as \textit{free}.
               \ELSIF{$|c^k| < C$}
                   \STATE Mark cluster $c^k$ as \textit{sparse}.
               \ENDIF
           \ENDFOR
           \STATE Reallocate all \textit{free} samples $x_j$ to their nearest \textit{sparse} cluster.
           \STATE Update centers of the novel clusters.
       \ENDFOR
   \end{algorithmic}
\end{algorithm}


%\begin{wrapfigure}{r}{0.4\textwidth}
%\begin{figure}[h]
\begin{figure*}[ht]
\begin{subfigure}{.24\textwidth}
  \centering
\centering
\resizebox{1\linewidth}{!}{
\begin{tikzpicture}
  % Overlapping blue cluster
  \draw[fill=blue, opacity=0.1] (1.25,0) ellipse (1.25cm and 1cm);

  % First realistic cluster with smaller red circles around z_i
\draw[fill=red, opacity=0.2] (0,0) circle (1cm);
  % Point z_i
  \filldraw [black] (0.5,0) circle (2pt) node[anchor=north] {$z_j$};

  % Second realistic cluster with smaller red circles around z_j
%\draw[fill=red, opacity=0.1] (3,0) circle (1cm);
  % Point z_j
  \filldraw [black] (2,0) circle (2pt) node[anchor=north] {$\mathbf{c_i}$};
  \node at (-0.25,0.5) {$k$};
\end{tikzpicture}}
\caption{}
  \label{fig:sfig1}
\end{subfigure}%
\begin{subfigure}{.24\textwidth}
  \centering
  \resizebox{1\linewidth}{!}{
\begin{tikzpicture}
  % Overlapping blue cluster
  \draw[fill=red, opacity=0.2] (1.25,0) ellipse (1.25cm and 1cm);

  % First realistic cluster with smaller red circles around z_i
\draw[fill=blue, opacity=0.1] (0,0) circle (0.75cm);
  % Point z_i
  \filldraw [black] (0.5,0) circle (2pt) node[anchor=north] {$z_j$};

  % Second realistic cluster with smaller red circles around z_j
\draw[fill=blue, opacity=0.1] (2,0) circle (1cm);
  % Point z_j
  \filldraw [black] (2,0) circle (2pt) node[anchor=north] {$\mathbf{c_i}$};
  \node at (0.9,0.5) {$k$};
\end{tikzpicture}}
  \caption{}
  \label{fig:sfig2}
\end{subfigure}
\begin{subfigure}{.24\textwidth}
  \centering
  \resizebox{1\linewidth}{!}{
\begin{tikzpicture}
  % Overlapping blue cluster
  \draw[fill=red, opacity=0.2] (1.25,0) ellipse (1.25cm and 1cm);

  % First realistic cluster with smaller red circles around z_i
\draw[fill=blue, opacity=0.1] (0,0) circle (0.75cm);
  % Point z_i
  \filldraw [black] (0.5,0) circle (2pt) node[anchor=north] {$z_j$};

  % Second realistic cluster with smaller red circles around z_j
\draw[fill=blue, opacity=0.1] (2,0) circle (1cm);
  % Point z_j
  \filldraw [black] (2,0) circle (2pt) node[anchor=north] {$z_i$};
  \node at (0.9,0.5) {$k$};
\end{tikzpicture}}
  \caption{}
  \label{fig:sfig3}
\end{subfigure}
\begin{subfigure}{.24\textwidth}
  \centering
  \resizebox{1\linewidth}{!}{
\begin{tikzpicture}
  % Overlapping blue cluster
  \draw[fill=blue, opacity=0.1] (1.25,0) ellipse (1.25cm and 1cm);

  % First realistic cluster with smaller red circles around z_i
\draw[fill=red, opacity=0.2] (0,0) circle (0.75cm);
  % Point z_i
  \filldraw [black] (0.5,0) circle (2pt) node[anchor=north] {$z_j$};

  % Second realistic cluster with smaller red circles around z_j
\draw[fill=red, opacity=0.2] (2,0) circle (1cm);
  % Point z_j
  \filldraw [black] (2,0) circle (2pt) node[anchor=north] {${z_i}$};
  \node at (-0.25,0.5) {$k$};
  \node at (2.5,0.5) {$l$};

\end{tikzpicture}}
  \caption{}
  \label{fig:sfig4}
\end{subfigure}
\caption{\textbf{Different scenarios for two sample context variables.} The latent variables $z_i$ and $z_j$ are extracted from the model and corresponds to the images $i$ and $j$, while ground truth context variable $\mathbf{c_i}$ is the groundtruth context variable for sample $i$. In the figures, red assignments are done by model, while blue assignments are the ground truth context variable assignments. There are multiple scenarios where the model makes a mistake in supervised contrastive learning in which only $i$'s label $\mathbf{c_i}$ is known. (a) Both $i$ and $j$ have the same labels; the model assigns $j$ to another label $k$. (b) $i$ and $j$ have different labels but $j$ is assigned to the label $k{=}\mathbf{c_i}$.
For unsupervised contrastive learning, neither of the labels is known, so the model makes a mistake if (c) $i$ and $j$ have different labels and are assigned to the same label $k$, (d) $i$ and $j$ have the same label, but model assign them to different labels $k$ and $l$. }%\cs{So? How are you going to fix it in this paper?}}
\label{fig:appclusters}
%\label{fig:bays}
%\end{figure}
\end{figure*}
%%%%%%%%%%%%%%%%%%%%%%%%%%%%%%%%%%%%
%GCD/NCD 2024
%%%%%%%%%%%%%%%%%%%%%%%%%%%%%%%%%%%%
\cite{liu2024novel} ultra fine Novel
\cite{colin2024practical} Tabular novel
\cite{rongali2024cdad} Domain gap GCD
\cite{ma2024active} active GCD
\cite{pu2024federated} Federated GCD
\cite{Cao_2024_CVPR} Solving the Catastrophic Forgetting Problem in Generalized Category Discovery
\cite{Xiao_2024_CVPR}Targeted Representation Alignment for Open-World Semi-Supervised Learning
\cite{Wu_2024_CVPR} ProTeCt: Prompt Tuning for Taxonomic Open Set Classification
\cite{Lang_2024_CVPR}From Coarse to Fine-Grained Open-Set Recognition
\cite{rypesc2024category} ECCV24

\cite{liu2024democratizing} Democratizing Fine-grained Visual Recognition with Large Language Models 
\cite{shi2024unified} 
\cite{zhou2024novel} Novel Class Discovery in Chest X-rays via Paired Images and Text
\cite{wang2024semantic}Semantic-Guided Novel Category Discovery
\cite{chen2024adaptive} Adaptive Discovering and Merging for Incremental Novel Class Discovery
\cite{feng2024debiased} Debiased Novel Category Discovering and Localization
\cite{an2024transfer} Transfer and alignment network for generalized category discovery

%%%%%%%%%%%%%%%%%%%%%%%%%%%%%%%%%%%%
%GCD/NCD 2023
%%%%%%%%%%%%%%%%%%%%%%%%%%%%%%%%%%%%
\cite{sun2024graph}A graph-theoretic framework for understanding open-world semi-supervised learning
\cite{weng2024decompose} Decompose Novel into Known: Part Concept Learning For 3D Novel Class Discovery

\cite{wang2024discover} Discover and align taxonomic context priors for open-world semi-supervised learning (TIDA)

\cite{yang2023generalized} Generalized category discovery with clustering assignment consistency
\cite{feng2023towards} Towards Novel Class Discovery: A Study in Novel Skin Lesions Clustering
\cite{zhang2023novel} Novel Class Discovery for Long-tailed Recognition
\cite{li2023generalized}Generalized Categories Discovery for Long-tailed Recognition

\cite{zang2023boosting} Boosting novel category discovery over domains with soft contrastive learning and all in one classifier

\cite{zheng2024textual}Textual Knowledge Matters: Cross-Modality Co-Teaching for Generalized Visual Class Discovery

\cite{li2023imbagcd} ImbaGCD: Imbalanced Generalized Category Discovery
\cite{hogan2023openworld}Open-world Semi-supervised Generalized Relation Discovery Aligned in a Real-world Setting
%%%%%%%%%%%%%%%%%%%%%%%%%%%%%%%%%%%%
%2022
%%%%%%%%%%%%%%%%%%%%%%%%%%%%%%%%%%%%
\cite{troisemaine2022method} A method for discovering novel classes in tabular data

\cite{an-etal-2022-fine} Fine-grained Category Discovery under Coarse-grained supervision with Hierarchical Weighted Self-contrastive Learning

\cite{rizve2022openldn} Openldn: Learning to discover novel classes for open-world semi-supervised learning

\cite{guo2022robust}Robust semi-supervised learning when not all classes have labels

%%%%%%%%%%%%%%%%%%%%%%%%%%%%%%%%%%%%
%SURVEY
%%%%%%%%%%%%%%%%%%%%%%%%%%%%%%%%%%%%

\cite{zhu2024open}Open-world machine learning: A review and new outlooks SURVEY

\cite{salehi2022a}
\cite{9723693}, A Survey on Open Set Recognition
\cite{boult2019learning}

\cite{kusupati2022matryoshka}Matryoshka representation learning
\cite{kim2020proxy} reviewer
\cite{yang2022hierarchical} reviewer
\cite{wu2017sampling} reviewer
%%%%%%%%%%%%%%%%%%%%%%%%%%%%%%%%%%%%
%Arxiv
%%%%%%%%%%%%%%%%%%%%%%%%%%%%%%%%%%%%

\cite{zhao2024labeled} Labeled Data Selection for Category Discovery
\cite{wang2024beyond} Beyond Known Clusters: Probe New Prototypes for Efficient Generalized Class Discovery
